# Supplementary material for: PGADA: Perturbation-Guided Adversarial Alignment for Few-shot Learning Under the Support-Query Shift
Source: arXiv:2205.03817 source file (2022-05-08)
Supplement: Supplementary file 2 [file setup.tex]

\section{Experiment Setup}\label{apx:setup}

\subsection{Datasets}

\begin{itemize}
    \item \textbf{CIFAR100.} We build a corrupted data set from CIFAR-100~\cite{krizhevsky2009learning}, which consists of $60,000$ three-channel square images of size $32 \times 32$, evenly distributed in $100$ classes. Classes are evenly distributed in $20$ superclasses.  We employee $19$ image transformations~\cite{zhang2020adaptive}, with $5$ levels of intensity, to evaluate the robustness of a model to the support-query shift. The training dataset, validation dataset, and testing dataset have $2,184,000$, $114,000$, $330,,000$ transformed images, respectively. For a fair comparison, we adopt the different transformations on each dataset to evaluate the robustness of our model.
    \item \textbf{miniImageNet.} We build a corrupted dataset from mini-ImageNet~\cite{triantafillou2019meta}, which contains $60,000$ three-channel square images of size $224 \times 224$ from $100$ classes from the ImageNet dataset with a $64$ classes training set, a $16$ classes validation set, and a $20$ classes test set~\cite{vinyals2016matching}. Same with~\cite{bennequin2021bridging}, we use $224 \times 224$ instead of $84 \times 84$ as our input image size. Similar to CIFAR100, miniImageNet also has the same transformations proposed by~\cite{hendrycks2019benchmarking} to simulate different domains~\cite{hendrycks2019benchmarking}. The training dataset, validation dataset, and testing dataset have $1,200,000$, $182,000$, $228,000$ transformed images, respectively. 
    \item \textbf{FEMNIST.} FEMNIST is the collection of handwritten digits and uppercase and lowercase characters, sorted by $3,500$ users. In the support-query shift few-shot learning setting, each group is built as a set of images written by one user. Note that in FEMNIST, most letters have less than two instances, although many users provide several instances for each digit. Therefore it is hard to find enough samples from a user to build a support set or a query set. As a result, experiments are limited to classification tasks with only one sample per class in both the support and query sets. At last, FEMNIST has $805,263$ handwritten characters $1$-channel square images of size $28 \times 28$ in $62$ classes ($42$ classes in training, $10$ classes invalidation, and $10$ classes in testing) consisting of different handwriting styles from $3,500$ users.
\end{itemize}

\subsection{Baseline}
The first five baselines are the state-of-the-art few-shot learning methods.
\begin{itemize}
    \item \textbf{MatchingNet~\cite{vinyals2016matching}.}  MatchingNet measures the pairwise cosine similarity between the support set and the query set and assigns the same class of the support example to the query example with the highest similarity.
    \item \textbf{ProtoNet~\cite{snell2017prototypical}.} Instead of pairwise similarity, ProtoNet uses euclidean distance to classify queries to the prototype embeddings, i.e., averaging the embeddings of all support examples in the same class. 
    \item \textbf{TransPropNet~\cite{liu2018learning}.} TransPropNet is an extension of ProtoNet, which utilizes a graph neural network to leverage information of local neighborhoods.
    \item \textbf{FTNET~\cite{dhillon2019baseline}.} FTNET is a meta-learning framework that estimates the distribution between the training set and testing set transductively.
    \item \textbf{TP~\cite{bennequin2021bridging}.} Transported Prototypes (TP) combines the ProtoNet, optimal transport, and transductive batch normalization to solve the support-query shift.
\end{itemize}
Our method is also closed to adversarial data augmentation. The second type of baselines contains $6$ state-of-the-art works related to this topic. 
\begin{itemize}
    \item \textbf{MixUp \cite{zhang2017mixup}.} MixUp creates virtual data points by mixing two samples with different opacity.
    \item \textbf{CutMix \cite{yun2019cutmix}.} CutMix  mixes different two samples by random crops.
    \item \textbf{Autoencoder \cite{schonfeld2019generalized}.} Autoencoder generate the augmented datas by minimizing the distance between the perturbed and origin embeddings.
    \item \textbf{AugGAN \cite{huang2018auggan}} AugGAN uses GAN to generate similar images as the data augmentation method.
    \item \textbf{MaxEntropy \cite{zhao2020maximum}.} MaxEntropy creates difficult data points following the maximum entropy.
    \item \textbf{MaxUp \cite{gong2021maxup}.} MaxUp samples the worst data point according to the original image and minimizing the empirical loss.
\end{itemize}

\subsection{Classifiers}
\label{appendix:nets}
In this section, we present the implementation detail of these two classifiers,i.e., MatchingNet~\cite{vinyals2016matching}, and ProtoNet~\cite{snell2017prototypical}, in the experiment.
\begin{itemize}

\item\textbf{Matching Network ~\cite{vinyals2016matching}.}
After obtaining representation from the embedding model $\phi$, Matching Network classifies each example $x_{q,j}$ in the query set $\mathcal{Q}$ to the class of the data point in the support set $\mathcal{S}$, with the highest cosine similarity. Given a support example $x^c_{s,i}$ for class $c$, the probability $p (y =c | x_{q,j}) $ is defined as follows.
\begin{equation*}
p (y =c | x_{q,j}) =  \frac{exp(cos(\phi(x_{q,j)},\phi(x^{c}_{s,i})))}{\sum_{\mathbf{c} \in \mathcal{C}} exp(cos(\phi(x^{\mathbf{c}}_{s,i}),\phi(x_{q,j)}))}.
\end{equation*}
Note that Matching Network only use one data point $x^c_{s,i}$ in the support set of class $c$ to classify the query set.

\item \textbf{Prototypical Network~\cite{snell2017prototypical} .}
Prototypical Network extends the Matching Network by introducing the prototype as there are multiple examples for each class in the support set. Formally, the prototype $\phi^{c}(x_{s,i})$ is defined as the mean vector of the support set in class $c$, i.e.,
\begin{align*}
\phi^{c}(x_{s}) = \frac{1}{|\mathcal{S}^c|} \sum_{x_{s,i} \in \mathcal{S}^c} (\phi(x_{s,i})).
\end{align*}
Then, The Euclidean distance is adopted to estimate the probability.
\begin{align*}
p (y =c | x_{q,j}) = \frac{exp(-\Vert{ \phi(x_{q,j}) - \phi^{c}(x_{s})}\Vert_2^{2})}{\sum_{\mathbf{c} \in C}exp(-\Vert{\phi(x_{q,j}) - \phi^{\mathbf{c}}(x_{s})}\Vert_2^{2}}) 
\end{align*}

\end{itemize}
