# Supplementary material for: PGADA: Perturbation-Guided Adversarial Alignment for Few-shot Learning Under the Support-Query Shift
Source: arXiv:2205.03817 source file (2022-05-08)
Supplement: Supplementary file 3 [file erm.tex]

\section{Effect of ERM and Episodic Training}
\label{appendix:erm}
