# Supplementary material for: PGADA: Perturbation-Guided Adversarial Alignment for Few-shot Learning Under the Support-Query Shift
Source: arXiv:2205.03817 source file (2022-05-08)
Supplement: Supplementary file 4 [file experiment.tex]

\section{Additional Experiment Results}
\label{apx:experiemnt}

\subsection{Effect of the Transductive Batch Normalization }
\label{appendix:tbncbn}
\begin{table*}[t]\small
\resizebox{\columnwidth}{!}{%
    \centering
    \begin{tabular}{ c|c|c|c|c|c|c|c|c|c }
\hline
  \multirow{3}*{Dataset}  &  \multicolumn{4}{|c|}{CIFAR100} &  \multicolumn{4}{|c|}{miniImageNet} & 
  FEMNIST\\

    \cline{2-10}
    &
    \multicolumn{2}{|c|}{8-target} &
    \multicolumn{2}{|c|}{16-target}&
    \multicolumn{2}{|c|}{8-target} &
    \multicolumn{2}{|c|}{16-target}&
    1-target \\
    \cline{2-10}
    & 1-shot& 5-shot & 
      1-shot& 5-shot & 
      1-shot& 5-shot & 
      1-shot& 5-shot & 
      1-shot \\
  \hline
  
  PGADA w/ TBN &  
 $\mathbf{42.16_{\pm 0.52}}$ &          $\mathbf{56.52_{\pm0.47}}$ &
 $\mathbf{42.73_{\pm 0.46}}$ & $\mathbf{56.83_{\pm0.40}}$ &
 $\mathbf{55.44_{\pm0.61}}$ &  $\mathbf{67.34_{\pm0.49}}$ &
 $\mathbf{55.69_{\pm0.62}}$ &  $\mathbf{66.90_{\pm0.50}}$ &
 $\mathbf{97.71_{\pm0.42}}$ \\
  
  PGADA w/ CBN & 
  $39.23_{\pm0.50}$ &
  $52.78_{\pm0.47}$ & 
  $39.75_{\pm0.45}$ & 
  $52.96_{\pm0.41}$ &
  $45.31_{\pm0.56}$ & 
  $57.42_{\pm0.48}$ &
  $45.63_{\pm0.50}$ & 
  $57.34_{\pm0.43}$ &
  $96.12_{\pm0.54}$ \\

%   PGADA$\dagger$ w/ TBN &   
%   $39.33_{\pm0.50}$& $53.66_{\pm0.47}$ &
%   $40.31_{\pm0.44}$& $54.23_{\pm0.40}$&
%   $47.96_{\pm0.57}$& $61.38_{\pm0.49}$&
%   $48.70_{\pm0.52}$& $61.44_{\pm0.43}$&
%   $96.53_{\pm0.52}$ \\

%     PGADA$\dagger$ w/ CBN &  
%  $39.72_{\pm0.51}$ &          
%  $53.18_{\pm0.46}$ &
%  $40.24_{\pm0.45}$ & 
%  $53.57_{\pm0.40}$ &
%  $48.44_{\pm0.59}$ &  
%  $60.91_{\pm0.50}$ &
%  $48.89_{\pm0.54}$ &  
%  $60.80_{\pm0.44}$ &
%  $96.03_{\pm0.55}$ \\
 
\hline    
\end{tabular}%
}
    \caption{Comparsion of TBN and CBN under the support-query shift. }
\label{table:tbn_cbn}
\end{table*}
% $\dagger$ means without self-supervised  loss.

Here, we explore the effect of transductive batch normalization (TBN)~\cite{bronskill2020tasknorm} and conventional batch normalization (CBN). TBN is first proposed in MAML~\cite{finn2017model}. Ren~\textit{et al.}\cite{ren2018meta} point out that TBN leverages a query set as a whole to bring a significant boost in performances compared to CBN. Therefore, we both deploy TBN and CBN to evaluate our method.  From Table~\ref{table:tbn_cbn}, we observe that PGADA gets unignorable benefit from TBN, which is consistent with prior works. Specifically, PGADA w/ TBN outperforms PGADA w/ CBN, $7.21\%$, $19.57\%$, $1.06\%$ on CIFAR100, miniImageNet, FEMNIST respectively. Once the self-supervised loss is removed, we observe that PGADA w/ TBN has a similar performance with PGADA w/ CBN.  It demonstrates that TBN and self-supervised learning can achieve better performance by exploring the inherent structure information from the unlabeled data.  Summing up, the prior works~\cite{finn2017model,triantafillou2019meta} point out that TBN is efficient in Meta-Learning, where TBN can explore whole query distribution cross tasks to achieve improvement. Our work obverse that the combination of TBN and self-supervised learning also performs well as they can learn more information from unlabeled data.  

% \input{experiment/case}

% Moreover, it shows that the generating the perturbed data  

% doesn't rely on TBN, but TBN with self-supervised learning .  

%  However, even with CBN, our method can still outperform prior works by a strong margin, which shows that our method doesn't only rely on TBN but also the robust embedding function derived from the augmented data we generate and inherent structure information from the unlabeled data. And therefore we find can that %One of the potential reasons is that TBN and self-supervised learning can combine well to learn the inherent structure information from the unlabeled data. 
