# Supplementary material for: PGADA: Perturbation-Guided Adversarial Alignment for Few-shot Learning Under the Support-Query Shift
Source: arXiv:2205.03817 source file (2022-05-08)
Supplement: Supplementary file 5 [file overview.tex]

\subsection{Architecture Overview}
\label{apx:overview}
\input{fig/representation}
