# Supplementary material for: PGADA: Perturbation-Guided Adversarial Alignment for Few-shot Learning Under the Support-Query Shift
Source: arXiv:2205.03817 source file (2022-05-08)
Supplement: Supplementary file 6 [file proof.tex]

\section{Proof}
\subsection{Proof of Lemma~\ref{lemma:err}}
The left side inequality immediately follows because $W$
is non-increasing under convolutions, since $\mathcal{N}_{\sqrt{\sigma_s^2+\sigma_q^2}}$ = $\mathcal{N}_{\sigma_s}*\mathcal{N}_{\sigma_q}$, where $*$ is the convolution operator. 

In the right side of the inequality, we adopt Kantorovich-Rubinstein duality to write the optimal transport as follows.
\begin{equation*}\small
    W(\mu_s,\mu_q) = \sup_{\Vert w \Vert_{Lip} \leq 1 } E_{\mu_s} [w] - \mathrm{E}_{\mu_q} [w]
\end{equation*}
\begin{equation*}\small
    W_\sigma(\mu_s,\mu_q) = \sup_{\Vert{w} \Vert_{Lip} \leq 1 } E_{\mu_s*\mathcal{N}_{\sigma_s}} [w_{\sigma}] - \mathrm{E}_{\mu_q*\mathcal{N}_{\sigma_q}} [w_{\sigma}]
\end{equation*}
where $\Vert{\cdot}\Vert_{Lip}$ is the Lipschitz norm. Letting  $w^{\ast}$ be optimal for $W(\mu_s,\mu_q)$, we obtain,
\begin{equation}\small
     W_\sigma(\mu_s,\mu_q) = \sup_{\Vert{\phi}\Vert_{Lip} \leq 1 } E_{\mu_s*\mathcal{N}_{\sigma_s}} [w^{\ast}] - \mathrm{E}_{\mu_q*\mathcal{N}_{\sigma_q}} [w^{\ast}].
    \label{eq:exp}
\end{equation}
Let $X_s\sim \mu_s$, $Z_s \sim {N_{\sigma_s}}$ as independent random variables, we have,
\begin{align}\small
    \label{eq:z_s}
     &| E_{\mu_s}[w^{\ast}] - E_{\mu_s*N_{\sigma_s}}[w^{\ast}] |\\  \nonumber
     = & E [w^{\ast} (X_s)] - E [w^{\ast} (X+Z_s)] \\
     \leq& E [\Vert{Z_s}\Vert_2^2] =  d \sigma_s. \nonumber
\end{align}
where the last in equality uses $\Vert{w^\ast}\Vert_{Lip} \leq 1$. $d$ is the dimension of the embedding vector. Similarly, $X_q\sim \mu_q$, $Z_q \sim {N_{\sigma_q}}$ as independent random variables, we have,
\begin{align}\small
    \label{eq:z_q}
     &| E_{\mu_q}[w^{\ast}] - E_{\mu_q*N_{\sigma_q}}[w^{\ast}] |\\  \nonumber \nonumber
     = & E [w^{\ast} (X_q)] - E [w^{\ast} (X+Z_q)] \\
    \leq & E [\Vert{Z_q}\Vert_2^2] =  d \sigma_q. \nonumber
\end{align}
By inserting Eq.~(\ref{eq:z_s}) and Eq.~(\ref{eq:z_q}) to Eq.~(\ref{eq:exp}), and Cauchy-Schwarz inequality,  we concludes the proof.
\label{appendix:Lemma1}

\subsection{Proof of Theorem~\ref{thm:err}}
\label{appendix:Theorem1}
Base on Lemma~\ref{lemma:err}, barycentric coordinate is defined as follows,
\begin{equation}\small
    \hat{\pi}^{\ast}_i = \frac{\pi^{\ast}(x_{s,i},x_{q,j}) }{ \sum_{x_{q,j}\in\mathcal{Q}}\pi^{\ast}(x_{s,i},x_{q,j})} \sim \mathcal{N}_{\sigma_s} 
    \label{eq:xi}
\end{equation}
Let $X_q\sim \mu_q$, $X^\sigma_q \sim {\mu_q * N_{\sigma_q}}$ as independent random variables, 
\begin{equation}\small
    E[X^{\sigma(t)}_q - X_q^{(t)}] = \sigma_q,
    \label{eq:err_q}
\end{equation}
where $X^{\sigma(t)}_q$ and $X_q^{(t)}$ denotes the $t$-th dimension of random variable $X^\sigma_q$ and $X_q$, respectively.

Combining Eq. (\ref{eq:xi}) and Eq. (\ref{eq:err_q}), the projected distribution $\hat{X}_s  \sim {\mu_s * N_{\sigma_s} * N_{\sigma_q}} = {\mu_s * N_{\sqrt{\sigma_s^2+\sigma_q^2}}}$.
\begin{equation}\small
    E[\hat{X}_s - X_s] = d\sqrt{\sigma_s^2 + \sigma_q^2}.
\end{equation}
The theorem follows.
